# Supplementary material for: Deep-learning-based coupled flow-geomechanics surrogate model for CO$_2$ sequestration
Source: arXiv:2105.01334 source file (2021-05-04)
Supplement: Supplementary file 1 [file appendix.tex]

\section*{Appendix A. Model Architecture Details}
\subsection*{Appendix A.1. Detailed R-U-Net Schematic}
%\textcolor{red}{[xxx - rev1, major comment 6]}
\textcolor{blue}{
The detailed R-U-Net architecture is illustrated in Fig.~\ref{fig:detailed-r-u-net-schematic}. The boxes correspond to multichannel feature maps and the colored arrows represent different operations. The gray arrow shows the copy and concatenation of the extracted features in the encoding net to the upsampled features in the decoding net. Specifically, `conv' in Fig.~\ref{fig:detailed-r-u-net-schematic} represents the convolutional blocks and `transposed-conv' denotes the transposed convolutional blocks. More details on these blocks as well as on the residual block are provided in Fig.~\ref{fig:operation-block}. }

\begin{figure}[H]
     \centering
     \begin{subfigure}[b]{1.2\textwidth}
         \centering
         \includegraphics[trim={0 2cm 0 3cm}, clip,width=\textwidth]{figs/appendix/R-U-Net-detailed-structure.pdf}
         %\caption{Saturation error accumulation comparison}
         %\label{fig:sat-map-error-accumulation}
     \end{subfigure}
    
    \caption{Detailed schematic for the R-U-Net. Each box denotes a multichannel feature map. The number of channels~$N_z$ is indicated above each box, and the values at the left of each box indicate corresponding feature map size~$N_x\times N_y$. The arrows denote the different operations. }
    \label{fig:detailed-r-u-net-schematic}
\end{figure}

\begin{figure}[H]
     \centering
     \begin{subfigure}[b]{0.32\textwidth}
         \centering
         \includegraphics[trim={5cm 3cm 5cm 3cm}, clip, width=\textwidth]{figs/appendix/conv_block.pdf}
         \caption{Conv block}
         \label{fig:conv-block}
     \end{subfigure}
     %\hfill
     \begin{subfigure}[b]{0.32\textwidth}
         \centering
         \includegraphics[trim={5cm 3cm 5cm 2cm}, clip, width=\textwidth]{figs/appendix/residual_block.pdf}
         \caption{Residual block}
         \label{fig:residual-block}
     \end{subfigure}
     %\hfill
     \begin{subfigure}[b]{0.32\textwidth}
         \centering
         \includegraphics[trim={5cm 3cm 5cm 3cm}, clip, width=\textwidth]{figs/appendix/transposed_conv.pdf}
         \caption{Transposed conv block}
         \label{fig:transposed-conv-block}
     \end{subfigure}

    \caption{Illustration of conv, residual and transposed conv blocks.}
    \label{fig:operation-block}
\end{figure}

%\textcolor{red}{[xxx - rev1, minor comment 10]}
\textcolor{blue}{As shown in Fig.~\ref{fig:operation-block}, conv represents a convolutional layer followed by batch normalization and ReLU nonlinear activation, while transposed conv denotes a transposed (upsampling) convolutional layer followed by a convolutional layer, batch normalization and ReLU. A stack of two convolutional layers with 128 filters of size $3\times3$ constitutes a residual block, in which the first convolutional layer has skip connections with the output of the second convolutional layer. }

\subsection*{Appendix A.2. Recurrent R-U-Net Architecture}
The detailed architecture of the recurrent R-U-Net is shown in Table~\ref{table:r-u-net architecture}. In the table, conv, transposed conv and residual block are as described in Appendix~A.1.
%\textcolor{red}{In the table, `Conv' represents a convolutional layer followed by batch normalization and ReLU nonlinear activation, while `Transposed conv' denotes a transposed (upsampling) convolutional layer followed by batch normalization and ReLU. A stack of two convolutional layers with 128 filters of size $3\times3\times128$ constitute a `Residual block,' in which the first convolutional layer has skip connections with the output of the second convolutional layer.} 
The convLSTM2D block, which also employs 128 filters of size $3\times3$, performs all of the LSTM gate operations. 
% The values of the different gates $\mathbf{f}^t$, $\mathbf{i}^t$, $\mathbf{o}^t$ and the proposed cell state~$\tilde{\mathbf{C}}^t$ are determined from the previous output state $\mathbf{H}^{t-1}$ and the current input $\boldsymbol\chi^t$. The specific expressions for these quantities are
% %
%  \begin{equation}
%      \mathbf{f}^t = \sigma(\mathbf{W}_{xf} * {\boldsymbol\chi}^t + \mathbf{W}_{hf}*\mathbf{H}^{t-1} + \mathbf{b}_f),
%  \end{equation}
%   \begin{equation}
%      \mathbf{i}^t = \sigma(\mathbf{W}_{xi} * {\boldsymbol\chi}^t + \mathbf{W}_{hi}*\mathbf{H}^{t-1} + \mathbf{b}_i),
%  \end{equation}
%   \begin{equation}
%      \mathbf{o}^t = \sigma(\mathbf{W}_{xo} * {\boldsymbol\chi}^t + \mathbf{W}_{ho}*\mathbf{H}^{t-1} + \mathbf{b}_o),
%  \end{equation}
%   \begin{equation}
%      \tilde{\mathbf{C}}^t = \tanh(\mathbf{W}_{xc} * {\boldsymbol\chi}^t + \mathbf{W}_{hc}*\mathbf{H}^{t-1} + \mathbf{b}_c).
%  \end{equation}
%  %
% In the above expressions, $\mathbf{W}$ and $\mathbf{b}$ are convolution filter weights and bias terms, which are both shared across convLSTM cells. The parameters associated with these quantities are tuned during the training process.
Note that the convLSTM net generates $(n_x/4, n_y/4, 128)$ activation maps for all $n_t$ time steps. The decoder layers process these $n_t$ activation maps separately to produce the state maps.

\begin{table}[H]
\begin{center}
\caption{Recurrent R-U-Net architecture details  %\textcolor{red}{[xxx - rev2, minor comment 10]}
}
  \label{table:r-u-net architecture}
  \begin{tabular}{ c | c | c  }
    \hline
    Net &  Layer  & Output size\\ 
     \hline
    \multirow{8}{4em}{Encoder}& Input  & $(n_x, n_y, 1)$ \\
    & conv, 16 filters of size $3\times3$, stride 2  & $(n_x/2, n_y/2, 16)$ \\
    & conv, 32 filters of size $3\times3$, stride 1  & $(n_x/2, n_y/2, 32)$ \\
    &conv, 64 filters of size $3\times3$, stride 2  & $(n_x/4, n_y/4, 64)$ \\
    &conv, 128 filters of size $3\times3$, stride 1  & $(n_x/4, n_y/4, 128)$ \\
    &residual block, 128 filters of size $3\times3$, stride 1& $(n_x/4, n_y/4, 128)$ \\
    &residual block, 128 filters of size $3\times3$, stride 1& $(n_x/4, n_y/4, 128)$ \\
    &residual block, 128 filters of size $3\times3$, stride 1& $(n_x/4, n_y/4, 128)$ \\ \hline
    ConvLSTM&convLSTM2D block, 128 filters of size $3\times3$, stride 1& $(n_x/4, n_y/4, 128, n_t)$ \\ \hline
    \multirow{8}{4em}{Decoder}&residual block, 128 filters of size $3\times3$, stride 1& $(n_x/4, n_y/4, 128, n_t)$ \\
    &residual block, 128 filters  of size $3\times3$, stride 1& $(n_x/4, n_y/4, 128, n_t)$ \\
    &residual block, 128 filters  of size $3\times3$, stride 1& $(n_x/4, n_y/4, 128, n_t)$ \\
    &transposed conv, 128 filters of size $3\times3$, stride 1  & $(n_x/4, n_y/4, 128, n_t)$ \\
    &transposed conv, 64 filters of size $3\times3$, stride 2  & $(n_x/2, n_y/2, 64, n_t)$ \\
    &transposed conv, 32 filters of size $3\times3$, stride 1  & $(n_x/2, n_y/2, 32, n_t)$ \\
    &tranposed conv, 16 filters of size $3\times3$, stride 2  & $(n_x, n_y, 16, n_t)$ \\
    &\textcolor{blue}{conv layer}, 1 filter of size $3\times3$, stride 1  & $(n_x, n_y, 1, n_t)$ \\
   
    \hline
  \end{tabular}
  \end{center}
\end{table}

\section*{Appendix B. Surrogate Model Results for a Four-Well Example}
%\textcolor{red}{[xxx - rev1, major comment 3, 5]}

\textcolor{blue}{In this appendix, we investigate the performance of the recurrent R-U-Net on a four-well binary channelized system. One of the realizations, along with the well locations, is shown in Fig.~\ref{fig:channel-60x60-wellloc}. The binary facies model and injection and production well locations are taken from Liu et al.~\cite{liu2019deep}. This setup involves hard data only at the four well locations. This corresponds to much less conditioning than in the 25-well example considered earlier.}

\textcolor{blue}{The problem specification is essentially the same as that described in Section~\ref{sect:setup}, though here the simulation time frame is 1500~days. We apply the same recurrent R-U-Net architecture, hyperparameter settings and training procedures as were used previously. A total of 500 new test cases are simulated using the surrogate and the numerical flow simulator. }

\textcolor{blue}{For this example we present saturation and pressure maps for the cases corresponding to the least, median and most cumulative water injection over the full simulation period. Results are shown, in Figs.~\ref{fig:channel60x60_sat} and \ref{fig:channel60x60_p}, at 1500~days. The top row displays the recurrent R-U-Net predictions, the middle row shows the AD-GPRS simulation results, and the bottom row indicates the difference. For both pressure and saturation, we see that the maps appear quite different for the three cases (in a very discrete sense for saturation), and that this variation is captured accurately by the surrogate model.}

%geomodels with least~($9.5\times 10^5\, \text{m}^3$), median~($1.3\times 10^6\, \text{m}^3$) and most~($1.6\times 10^6\, \text{m}^3$) accumulative injected water, 

\begin{figure}[H]
     \centering
     \begin{subfigure}[b]{0.5\textwidth}
         \centering
         \includegraphics[width=\textwidth]{figs/appendix/channel-60x60-wellloc-demo.png}
         %\caption{Saturation error accumulation comparison}
         %\label{fig:sat-map-error-accumulation}
     \end{subfigure}
    
    \caption{Channelized $60\times60$ facies map, conditioned to facies type at four wells. White circles denote production wells and white triangles indicate injection wells. Model is from \cite{liu2019deep}.}
    \label{fig:channel-60x60-wellloc}
\end{figure}

\begin{figure}
     \centering
     \begin{subfigure}[b]{0.325\textwidth}
         \centering
         \includegraphics[width=\textwidth]{figs/appendix/ind_case_286_sat_step10.png}
         \caption{least water injected}
         \label{fig:sat-map-single-step1}
     \end{subfigure}
     %\hfill
     \begin{subfigure}[b]{0.325\textwidth}
         \centering
         \includegraphics[width=\textwidth]{figs/appendix/ind_case_443_sat_step10.png}
         \caption{median water injected}
         \label{fig:sat-map-single-step4}
     \end{subfigure}
     %\hfill
     \begin{subfigure}[b]{0.325\textwidth}
         \centering
         \includegraphics[width=\textwidth]{figs/appendix/ind_case_259_sat_step10.png}
         \caption{most water injected}
         \label{fig:sat-map-single-step9}
     \end{subfigure}
    \caption{Saturation maps from recurrent R-U-Net surrogate model (top row) and numerical simulator (middle row), along with difference maps (bottom row), for the test-set geomodels with (a) least, (b) median and (c) most cumulative water injected over the 1500-day simulation time frame.}
    \label{fig:channel60x60_sat}
\end{figure}

\begin{figure}
     \centering
     \begin{subfigure}[b]{0.325\textwidth}
         \centering
         \includegraphics[width=\textwidth]{figs/appendix/ind_case_286_p_step10.png}
         \caption{least water injected}
         \label{fig:sat-map-single-step1}
     \end{subfigure}
     %\hfill
     \begin{subfigure}[b]{0.325\textwidth}
         \centering
         \includegraphics[width=\textwidth]{figs/appendix/ind_case_443_p_step10.png}
         \caption{median water injected}
         \label{fig:sat-map-single-step4}
     \end{subfigure}
     %\hfill
     \begin{subfigure}[b]{0.325\textwidth}
         \centering
         \includegraphics[width=\textwidth]{figs/appendix/ind_case_259_p_step10.png}
         \caption{most water injected}
         \label{fig:sat-map-single-step9}
     \end{subfigure}
    \caption{Pressure maps from recurrent R-U-Net surrogate model (top row) and numerical simulator (middle row), along with difference maps (bottom row), for the test-set geomodels with (a) least, (b) median and (c) most cumulative water injected over the 1500-day simulation time frame.}
    \label{fig:channel60x60_p}
\end{figure}

\textcolor{blue}{Finally, we compare the accuracy of the recurrent R-U-Net and autoregressive DenseED surrogate models for pressure and saturation predictions in this four-well example. The pressure normalization described in Section~\ref{sect:data_proc} is applied for both surrogate models, and we set $\lambda=0$ in Eq.~\ref{eq:loss-function}. Errors are again computed using Eqs.~\ref{eq:sat-relative-error-time-t} and \ref{eq:pressure-relative-error-time-t}. Results are shown in Fig.~\ref{fig:state-map-error-accumulation-channel60x60}. We again see that our recurrent R-U-Net provides generally lower error (though autoregressive DenseED is more accurate for pressure at early time) and that this error grows only slowly in time. These results are consistent with those presented earlier for the 25-well example.}

\begin{figure}
     \centering
     \begin{subfigure}[b]{0.6\textwidth}
         \centering
         \includegraphics[width=\textwidth]{figs/appendix/Channel60x60MeanSaturationRelativeErrorInjSameSide.pdf}
         \caption{Saturation error}
         \label{fig:sat-map-error-accumulation-channel60x60}
     \end{subfigure}
     %\hfill
     \begin{subfigure}[b]{0.6\textwidth}
         \centering
         \includegraphics[width=\textwidth]{figs/appendix/Channel60x60MeanPressureRelativeErrorInjSameSide.pdf}
         \caption{Pressure error}
         \label{fig:p-map-error-accumulation-channel60x60}
     \end{subfigure}
    
    \caption{Relative saturation error $\delta_S^t$~(Eq.~\ref{eq:sat-relative-error-time-t}) and pressure error $\delta_p^t$~(Eq.~\ref{eq:pressure-relative-error-time-t}) at different time steps using the recurrent R-U-Net and autoregressive DenseED \citep{mo2018deep} procedures for the four-well channelized system.}
    \label{fig:state-map-error-accumulation-channel60x60}
\end{figure}
